# Supplementary material for: Acoustic characterization of speech rhythm: going beyond metrics with recurrent neural networks
Source: arXiv:2401.14416 source file (2024-01-22)
Supplement: Supplementary file 1 [file SI_all.pdf]

# Acoustic characterization of speech rhythm: Supplementary Information

## Contents

Supplementary information on the datasets . . . 2
Full confusion matrix . . . 7
Hierarchical clustering dendograms . . . 9
Additional figures for the comparison of features with rhythm metrics . . . 10
Individual cell activations . . . 10
Correlates with ElasticNet . . . 12
Results for a second version of the DNN . . . 13

## Supplementary information on the datasets

| Language\Dataset | librivox | CommonVoice | voxforge | WLI | tatoeba | TRAIN | % TRAIN | % TOTAL |
|---|---|---|---|---|---|---|---|---|
| German | 6,884 | 59,195 | 743 | 1,278 | 1,724 | 69,824 | 16.96% | 15.63% |
| English | 6,637 | 47,861 | 6,109 | 1,202 | 127 | 61,936 | 15.05% | 13.87% |
| French | 2,121 | 44,561 | 870 | 3,842 | 702 | 52,096 | 12.66% | 11.66% |
| Catalan | 0 | 44,576 | 0 | 1,376 | 0 | 45,952 | 11.16% | 10.29% |
| Spanish | 5,515 | 27,598 | 2,681 | 3,635 | 1,435 | 40,864 | 9.93% | 9.15% |
| Italian | 6,450 | 15,962 | 1,055 | 4,597 | 0 | 28,064 | 6.82% | 6.28% |
| Basque | 0 | 14,742 | 0 | 122 | 0 | 14,864 | 3.61% | 3.33% |
| Russian | 3,452 | 6,536 | 1,342 | 490 | 228 | 12,048 | 2.93% | 2.70% |
| Mandarin | 3,012 | 7,072 | 0 | 1,501 | 367 | 11,952 | 2.90% | 2.68% |
| Portuguese | 2,778 | 2,576 | 271 | 6,263 | 0 | 11,888 | 2.89% | 2.66% |
| Korean | 1,455 | 0 | 0 | 8,737 | 0 | 10,192 | 2.48% | 2.28% |
| Swedish | 3,346 | 707 | 0 | 4,923 | 0 | 8,976 | 2.18% | 2.01% |
| Dutch | 2,657 | 5,192 | 438 | 0 | 113 | 8,400 | 1.33% | 1.22% |
| Finnish | 3,830 | 0 | 0 | 3,418 | 0 | 7,248 | 1.76% | 1.62% |
| Polish | 3,714 | 0 | 0 | 1,714 | 28 | 5,456 | 1.33% | 1.22% |
| Danish | 1,599 | 0 | 0 | 3,617 | 0 | 5,216 | 1.27% | 1.17% |
| Arabic | 0 | 1,363 | 0 | 2,797 | 0 | 4,160 | 1.01% | 0.93% |
| Turkish | 0 | 2,975 | 233 | 712 | 0 | 3,920 | 0.95% | 0.88% |
| Estonian | 0 | 2,598 | 0 | 154 | 0 | 2,752 | 0.67% | 0.62% |
| Japanese | 1,617 | 365 | 0 | 536 | 202 | 2,720 | 0.66% | 0.61% |
| Hungarian | 755 | 0 | 0 | 1,503 | 94 | 2,352 | 0.57% | 0.53% |
| Romanian | 0 | 0 | 0 | 640 | 0 | 640 | 0.16% | 0.14% |
| Czech | 0 | 0 | 0 | 96 | 0 | 96 | 0.02% | 0.02% |
| TOTAL | 55,822 | 283,879 | 13,742 | 53,153 | 5,020 | 411,616 | 100.00% | **92.15%** |
| | 13.56% | 68.97% | 3.34% | 12.91% | 1.22% | 100.00% | | |

**Supplementary Table Supp. 1**: Number of 10-second samples by language and database in the **training** set. Note: Czech and Romanian were not used for training because of too few samples.

| Language\Dataset | librivox | CommonVoice | voxforge | WLI | tatoeba | TEST | % TEST | % TOTAL |
|---|---|---|---|---|---|---|---|---|
| German | 693 | 609 | 626 | 615 | 1 | 2,544 | 7.25% | 0.57% |
| English | 738 | 621 | 607 | 610 | 0 | 2,576 | 7.34% | 0.58% |
| French | 693 | 650 | 597 | 658 | 122 | 2,720 | 7.75% | 0.61% |
| Catalan | 0 | 624 | 0 | 0 | 0 | 624 | 1.78% | 0.14% |
| Spanish | 702 | 623 | 600 | 769 | 26 | 2,720 | 7.75% | 0.61% |
| Italian | 893 | 641 | 610 | 208 | 0 | 2,352 | 6.70% | 0.53% |
| Basque | 0 | 609 | 0 | 127 | 0 | 736 | 2.10% | 0.16% |
| Russian | 726 | 644 | 607 | 575 | 280 | 2,832 | 8.07% | 0.63% |
| Mandarin | 645 | 654 | 0 | 749 | 0 | 2,048 | 5.84% | 0.46% |
| Portuguese | 771 | 624 | 303 | 526 | 0 | 2,224 | 6.34% | 0.50% |
| Korean | 52 | 0 | 0 | 652 | 0 | 704 | 2.01% | 0.16% |
| Swedish | 213 | 498 | 0 | 633 | 0 | 1,344 | 3.83% | 0.30% |
| Dutch | 793 | 619 | 618 | 0 | 210 | 2,240 | 3.92% | 0.31% |
| Finnish | 322 | 0 | 0 | 750 | 0 | 1,072 | 3.06% | 0.24% |
| Polish | 493 | 0 | 0 | 883 | 0 | 1,376 | 3.92% | 0.31% |
| Danish | 255 | 0 | 0 | 577 | 0 | 832 | 2.37% | 0.19% |
| Arabic | 0 | 635 | 0 | 725 | 0 | 1,360 | 3.88% | 0.30% |
| Turkish | 0 | 621 | 231 | 604 | 0 | 1,456 | 4.15% | 0.33% |
| Estonian | 0 | 598 | 0 | 170 | 0 | 768 | 2.19% | 0.17% |
| Japanese | 198 | 373 | 0 | 516 | 49 | 1,136 | 3.24% | 0.25% |
| Hungarian | 11 | 0 | 0 | 653 | 8 | 672 | 1.92% | 0.15% |
| Romanian | 0 | 0 | 0 | 640 | 0 | 640 | 1.82% | 0.14% |
| Czech | 0 | 0 | 0 | 112 | 0 | 112 | 0.32% | 0.03% |
| TOTAL | 8,198 | 9,643 | 4,799 | 11,752 | 696 | 35,088 | 100.00% | **7.85%** |
| | 23.36% | 27.48% | 13.68% | 33.49% | 1.98% | 100.00% | | |

**Supplementary Table Supp. 2**: Number of 10-second samples by language and database in the **test** set.

| Language\Dataset | Librivox | CommonVoice | VoxForge | WLI | Tatoeba | TOTAL | % TOTAL |
|---|---|---|---|---|---|---|---|
| German | 7,577 | 59,804 | 1,369 | 1,893 | 1,725 | 72,368 | 16.20% |
| English | 7,375 | 48,482 | 6,716 | 1,812 | 127 | 64,512 | 14.44% |
| French | 2,814 | 45,211 | 1,467 | 4,500 | 824 | 54,816 | 12.27% |
| Catalan | 0 | 45,200 | 0 | 1,376 | 0 | 46,576 | 10.43% |
| Spanish | 6,217 | 28,221 | 3,281 | 4,404 | 1,461 | 43,584 | 9.76% |
| Italian | 7,343 | 16,603 | 1,665 | 4,805 | 0 | 30,416 | 6.81% |
| Basque | 0 | 15,351 | 0 | 249 | 0 | 15,600 | 3.49% |
| Russian | 4,178 | 7,180 | 1,949 | 1,065 | 508 | 14,880 | 3.33% |
| Mandarin | 3,657 | 7,726 | 0 | 2,250 | 367 | 14,000 | 3.13% |
| Portuguese | 3,549 | 3,200 | 574 | 6,789 | 0 | 14,112 | 3.16% |
| Korean | 1,507 | 0 | 0 | 9,389 | 0 | 10,896 | 2.44% |
| Swedish | 3,559 | 1,205 | 0 | 5,556 | 0 | 10,320 | 2.31% |
| Dutch | 3,450 | 5,811 | 1,056 | 0 | 323 | 10,640 | 2.38% |
| Finnish | 4,152 | 0 | 0 | 4,168 | 0 | 8,320 | 1.86% |
| Polish | 4,207 | 0 | 0 | 2,597 | 28 | 6,832 | 1.53% |
| Danish | 1,854 | 0 | 0 | 4,194 | 0 | 6,048 | 1.35% |
| Arabic | 0 | 1,998 | 0 | 3,522 | 0 | 5,520 | 1.24% |
| Turkish | 0 | 3,596 | 464 | 1,316 | 0 | 5,376 | 1.20% |
| Estonian | 0 | 3,196 | 0 | 324 | 0 | 3,520 | 0.79% |
| Japanese | 1,815 | 738 | 0 | 1,052 | 251 | 3,856 | 0.86% |
| Hungarian | 766 | 0 | 0 | 2,156 | 102 | 3,024 | 0.68% |
| Romanian | 0 | 0 | 0 | 1,280 | 0 | 1,280 | 0.29% |
| Czech | 0 | 0 | 0 | 208 | 0 | 208 | 0.05% |
| TOTAL | 64,020 | 293,522 | 18,541 | 64,905 | 5,716 | 446,704 | 100.00% |
| | 14.33% | 65.71% | 4.15% | 14.53% | 1.28% | 100.00% | |

**Supplementary Table Supp. 3**: Number of 10-second samples by language and database (synthesis).

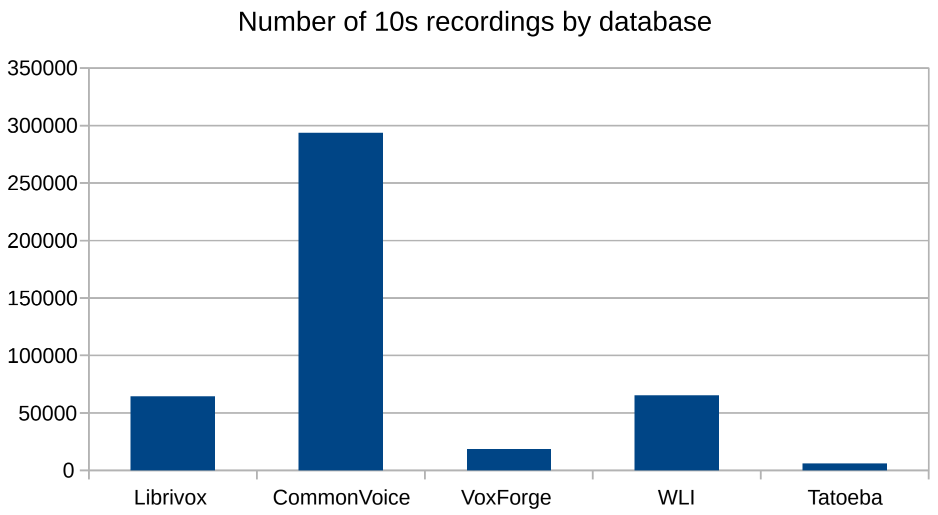


**Supplementary Figure Supp. 4**: Number of 10-second samples by database.

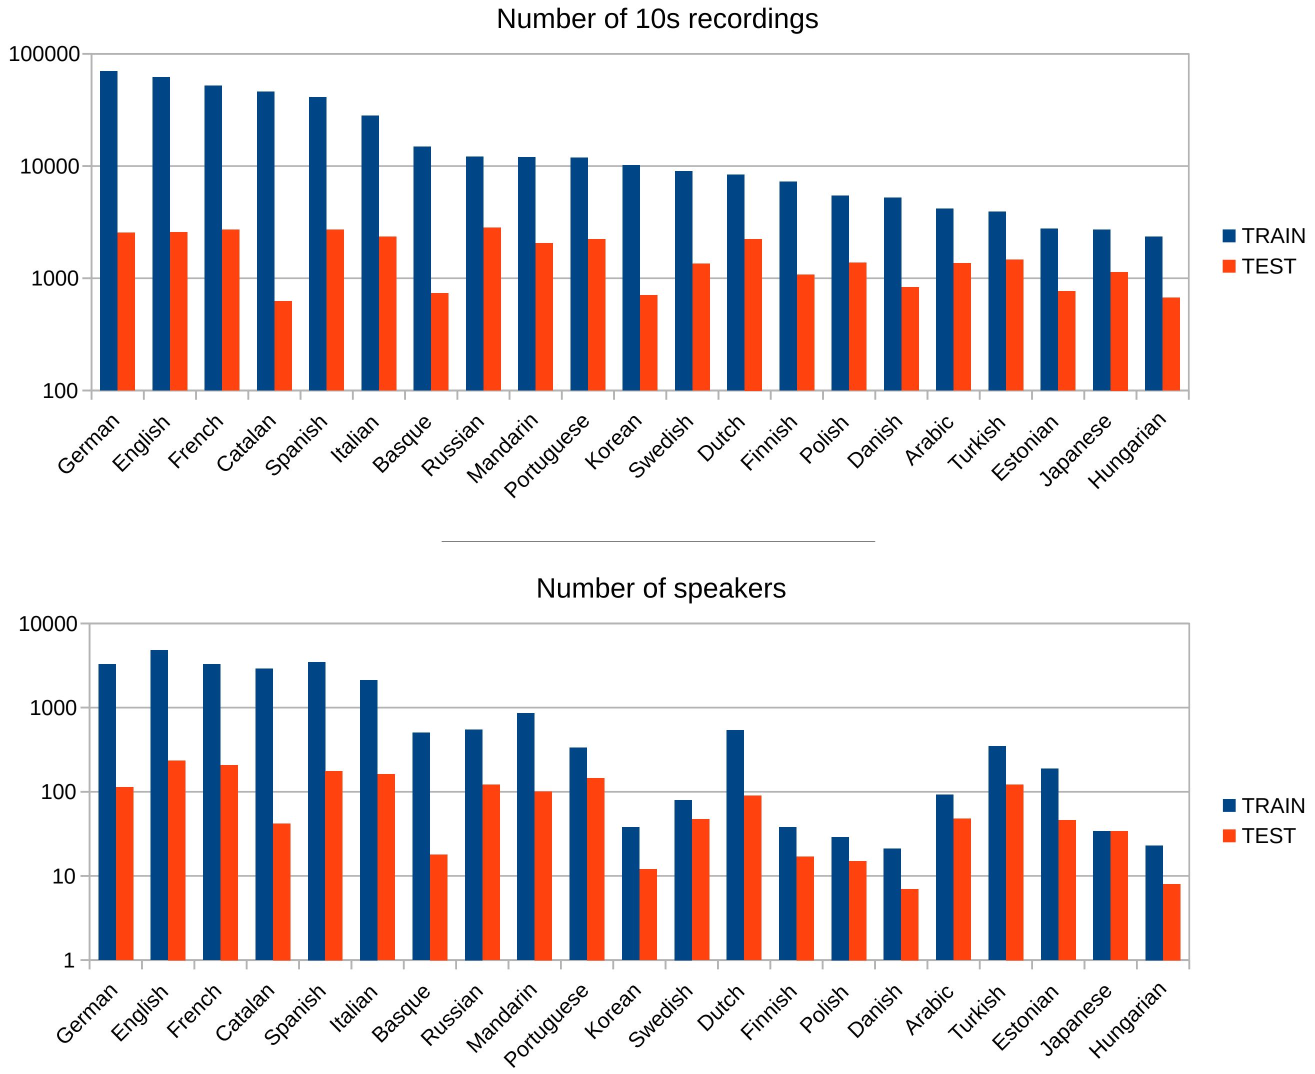


**Supplementary Figure Supp. 5**: Number of 10-second samples and approximated number of speakers by language (logarithmic scale).

### Full confusion matrix

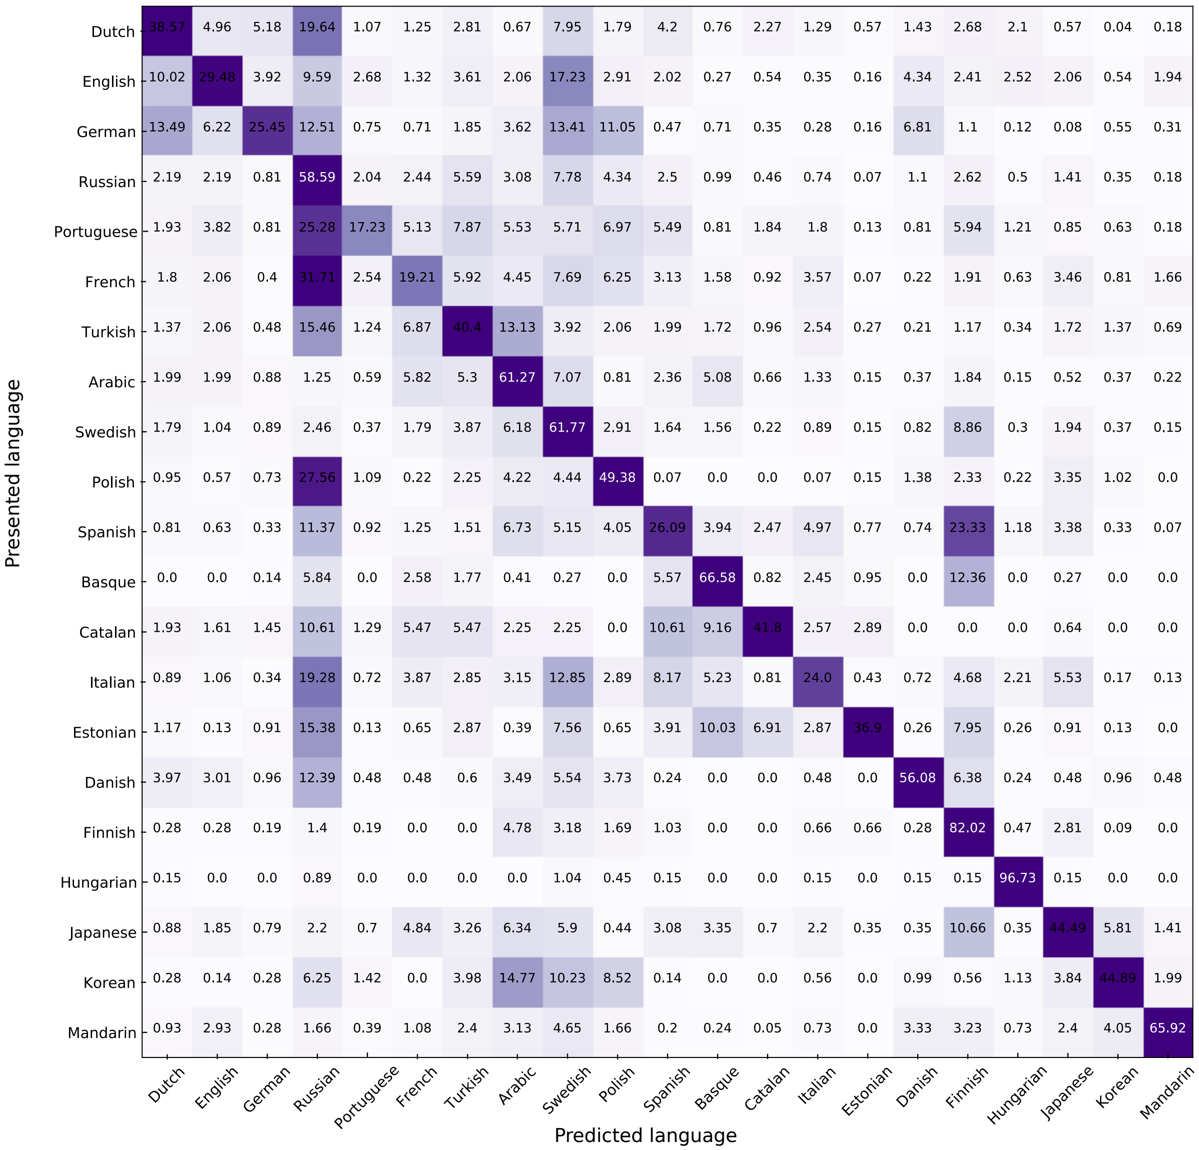


**Supplementary Figure Supp. 6**: Full confusion matrix (same model as in paper) considering all the languages of the dataset. Note that the network is biased in misclassifying examples as ‘Russian’. Other versions of the model (with different hyper-parameters) presented the same bias issue but not always with Russian.

## Hierarchical clustering dendograms

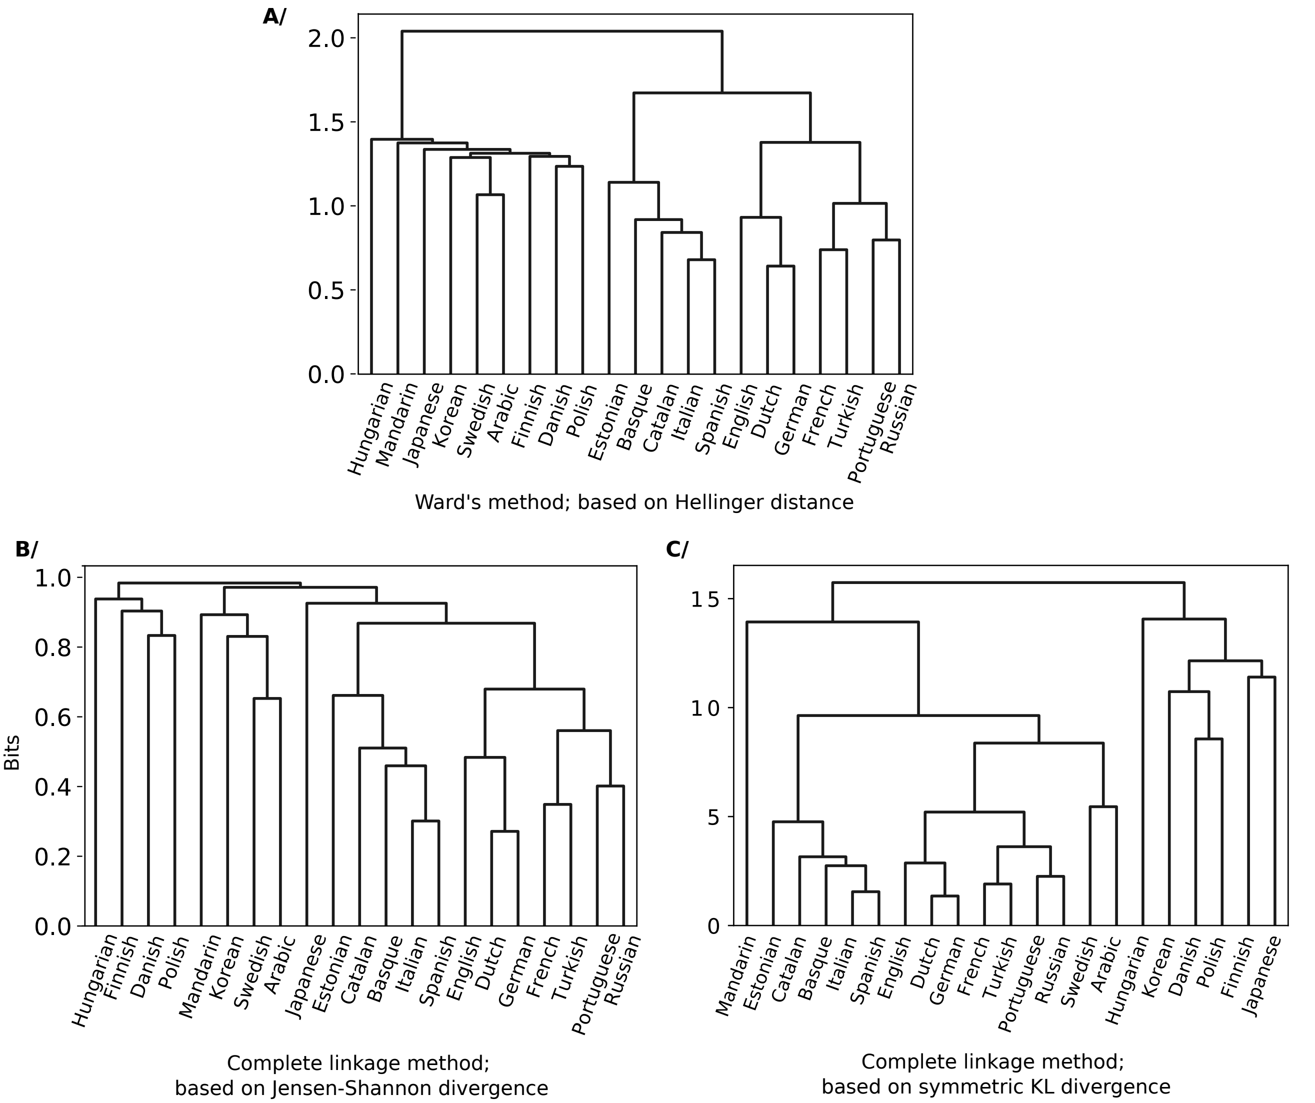


**Supplementary Figure Supp. 7**: Hierarchical clustering dendograms based on histograms of the DNN probability vector output (same model version as in paper) using different linkage methods or divergence measures: **A/** Ward's linkage method using Hellinger distance. **B and C/** Complete linkage methods using information-theoretic divergence measures.

## Additional figures for the comparison of features with rhythm metrics

### Individual cell activations

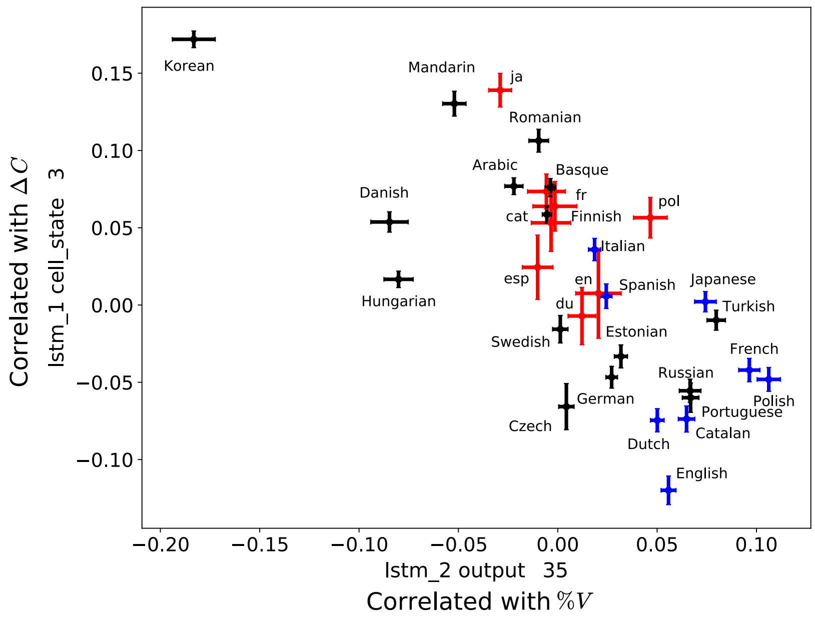


**Supplementary Figure Supp. 8**: Map based on activations of cells most correlated with $\%V$ (layer 2, cell 35, r=0.5) and $\Delta C$ (layer 1, cell 3, r=0.45) on the Ramus et al. corpus. Error bars correspond to standard error, for data averaged over the Ramus et al. corpus (red crosses, short form labels) and over 7,000 recordings from the current dataset (blue and black crosses). Note that the generalization error is important for this particular example, according to the distance between blue and red crosses.

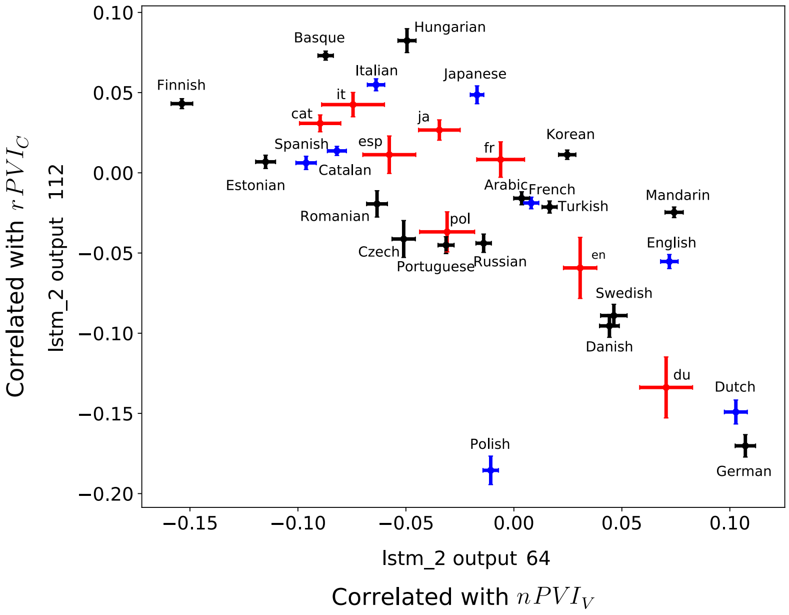


**Supplementary Figure Supp. 9**: Map based on activations of cells most correlated with $nPVI_V$ (layer 2, cell 64, r=0.47) and $rPVI_C$ (layer 2, cell 112, r=0.4) on the Ramus et al. corpus.

**Correlates with ElasticNet**

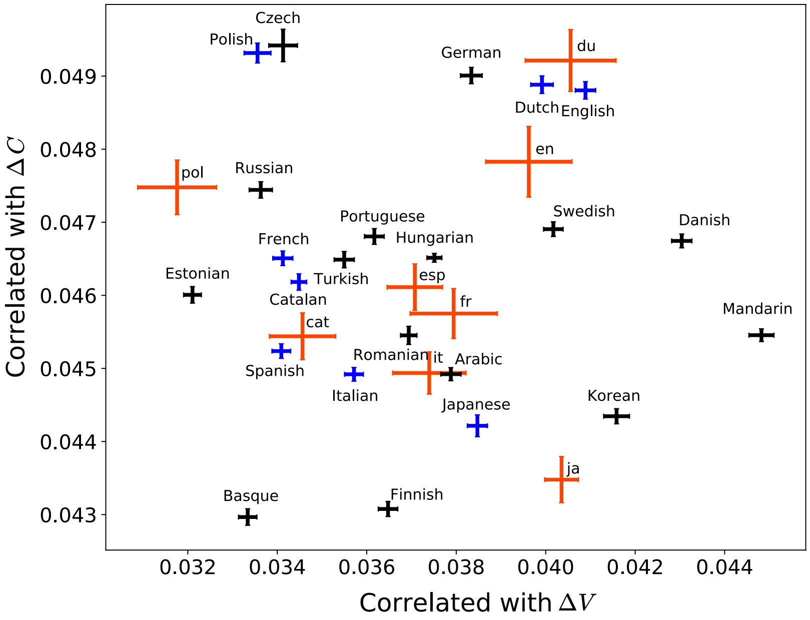


**Supplementary Figure Supp. 10**: Maps based on features (hidden layer activations) correlated with $(\Delta V, \Delta C)$ (found with ElasticNet on the Ramus et al. corpus)

### Results for a second version of the DNN

In this section, Results are shown for a larger version of the network $F_0$ as third input feature instead of the voicing information. This version is more accurate in discriminating languages but have more independent clusters using visualization methods complicating its analysis.

- Architecture (hidden layers): 2x180
- features: SPL, SPL-H, F0
- dropout: 0.2 (standard, applied to hidden layers only)
- number of epochs: 30
- Accuracy on test set: 61% (top-3 accuracy: 82%)

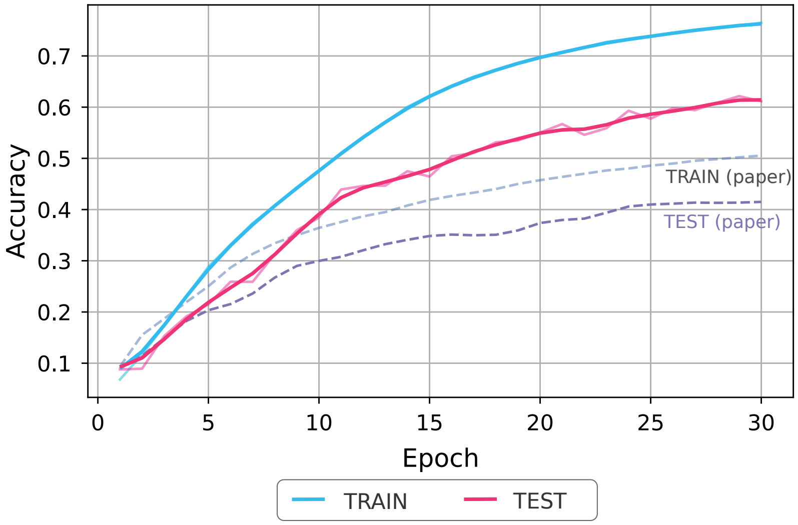


**Supplementary Figure Supp. 11**: Model accuracy as a function of epoch on train and test sets (values for the model shown in paper are given for reference).

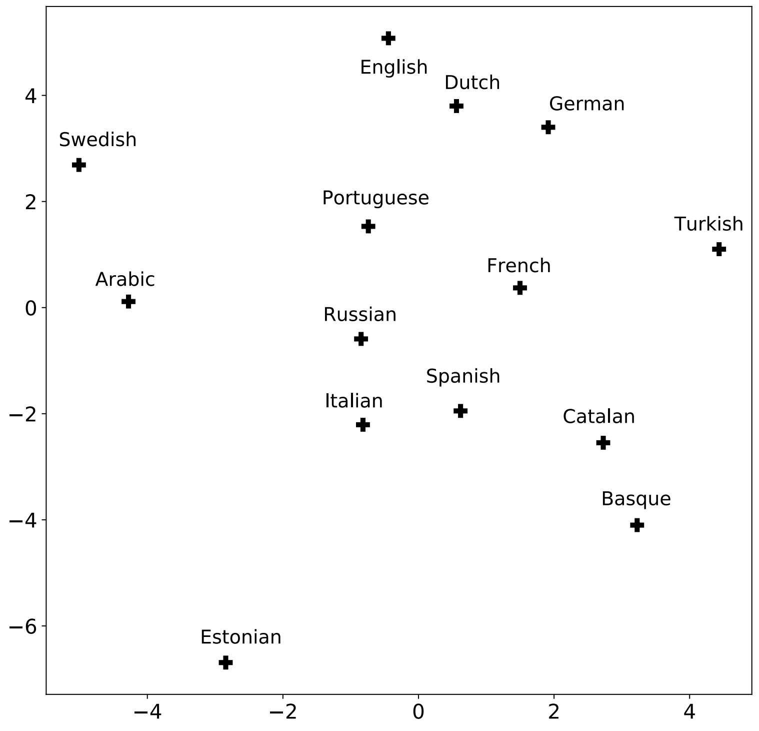


**Supplementary Figure Supp. 12**: MDS with output vector activation histograms and the Bhattacharyya distance (selected languages (see main text), stress: 0.19). One of the main differences with the version presented in the paper is the independent cluster formed by Estonian.

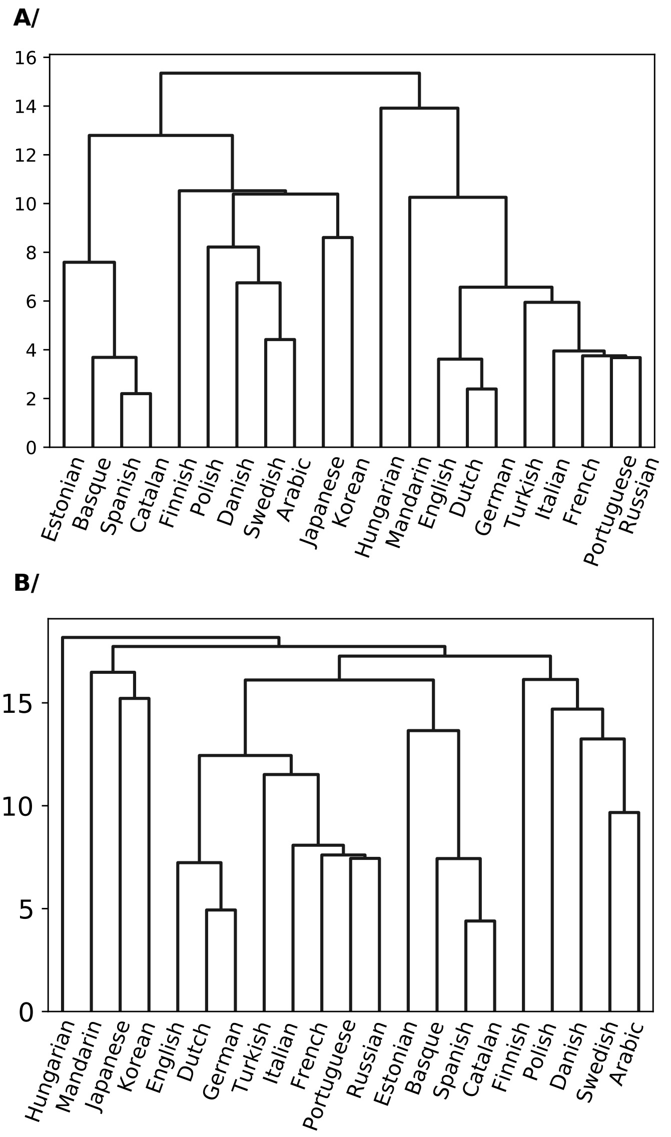


**Supplementary Figure Supp. 13**: Hierarchical clustering dendogram for the enlarged model based on histograms of the DNN probability vector output using the complete linkage method and Bhattacharyya distance (A/) or symmetric KL divergence (B/).

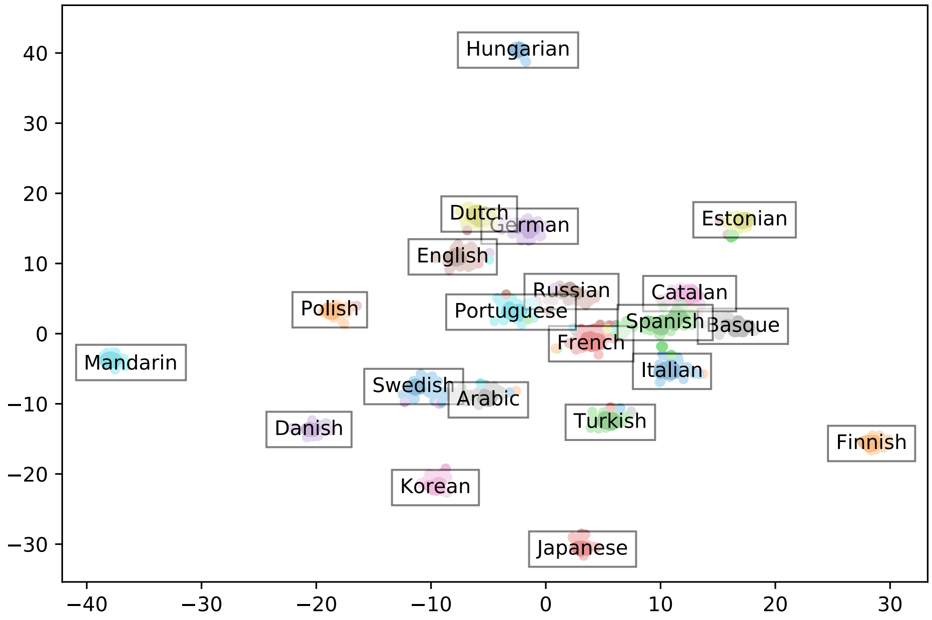


**Supplementary Figure Supp. 14**: One output of the t-SNE algorithm for the enlarged model on output probability vectors using the Hellinger distance (colors represent predicted language).

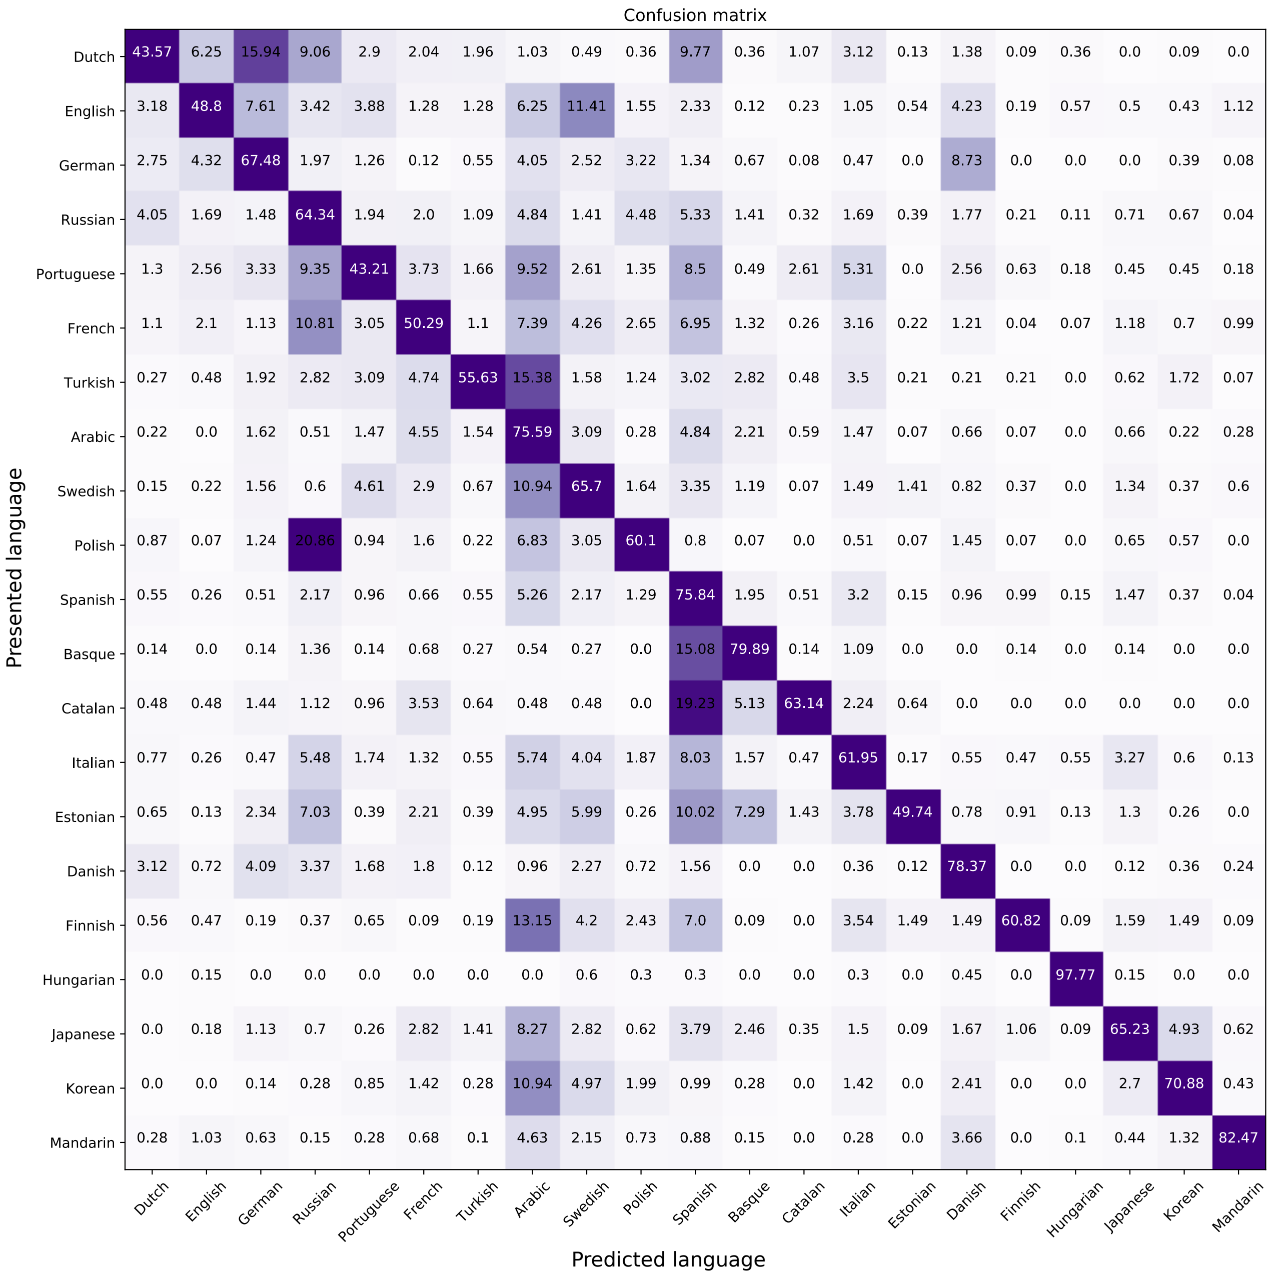


**Supplementary Figure Supp. 15**: Confusion matrix on the test set for the enlarged model.
